# Supplementary material for: Prioritizing Informative Features and Examples for Deep Learning from Noisy Data
Source: arXiv:2403.00013 source file (2024-08-12)
Supplement: Supplementary file 1 [file 7_appendix.tex]

\section{Supplementary Material}

%%%TODO: move std to the corresponding original tables

\subsection{Details of Experiment Results}
WILL MOVE STD TO THE CORRESPONDING ORIGINAL TABLES.

\begin{table}[t!]
\caption{Classification accuracy and standard deviation\,($\%$) of \algnamea{} on two CIFARs\,(32$\times$32), ImageNet-10\,(64$\times$64), and ImageNet-10\,(224$\times$224).} 
\begin{center}
\small
\begin{tabular}{X{1.5cm} |X{1.4cm} |X{1.5cm} X{1.5cm} X{1.5cm} X{1.5cm} X{1.5cm}} \toprule
\multicolumn{2}{c|}{{Datasets}} & \multicolumn{5}{c}{{\# Examples ($N$)}} \\\cline{1-2}\cline{3-7}\Tstrut
In-dist. &\!\!OOD\!\!& 500 &  1,000 & 2,500  & 5,000 & Full-shot \\ \midrule
% contetns
\multirow{2}{*}{\vspace*{-0.cm}\makecell[c]{CIFAR-10\\ (32$\times$32)}}
& SVHN&\!\!41.58$\pm$0.15\!\!&\!\!56.72$\pm$0.10\!\!&\!\!73.61$\pm$0.07\!\!&\!\!82.88$\pm$0.05\!\!&\!\!94.45$\pm$0.02\!\!\\\cline{2-7}\Tstrut
& {LSUN} &\!\!{\textbf{42.51}$\pm$0.11}\!\!&\!\!{\textbf{56.79}$\pm$0.05}\!\!&\!\!{\textbf{74.15}$\pm$0.04}\!\!&\!\!{\textbf{83.73}$\pm$0.02}\!\!&\!\!{\textbf{95.02}$\pm$0.03}\!\!\\ \midrule
\multirow{2}{*}{\vspace*{-0.cm}\makecell[c]{CIFAR-100\\(32$\times$32)}}
&SVHN&\!\!11.30$\pm$0.14\!\!&\!\!15.13$\pm$0.21\!\!&\!\!24.91$\pm$0.07\!\!&\!\!43.61$\pm$0.05\!\!&\!\!75.38$\pm$0.03\!\!\\ \cline{2-7}\Tstrut
& {LSUN} &\!\!{\textbf{12.26}$\pm$0.09}\!\!&\!\!{\textbf{15.97}$\pm$0.07}\!\!&\!\!{\textbf{25.36}$\pm$0.04}\!\!&\!\!{\textbf{44.50}$\pm$0.04}\!\!&\!\!{\textbf{75.69}$\pm$0.02}\!\!\\ \midrule  
\multirow{2}{*}{\vspace*{-0.05cm}\makecell[c]{\!\!\!ImgNet-10\!\!\!\\ (64$\times$64)}}
&\!\!\!ImgNet-990\!\!\!&\!\!42.80$\pm$0.11\!\!&\!\!46.04$\pm$0.10\!\!&\!\!\textbf{60.40}$\pm$0.07\!\!&\!\!\textbf{70.51}$\pm$0.04\!\!&\!\!\textbf{81.09}$\pm$0.03\!\!\\ \cline{2-7}\Tstrut
& Places365 &\!\!\textbf{43.25}$\pm$0.07\!\!&\!\!\textbf{47.61}$\pm$0.08\!\!&\!\!60.02$\pm$0.07\!\!&\!\!68.25$\pm$0.06\!\!&\!\!80.89$\pm$0.04\!\!\\ \midrule
\multirow{2}{*}{\vspace*{-0.05cm}\makecell[c]{\!\!\!ImgNet-10\!\!\!\\(224$\times$224)}}
&\!\!\!ImgNet-990\!\!\!&\!\!48.39$\pm$0.20\!\!&\!\!59.06$\pm$0.15\!\!&\!\!76.47$\pm$0.06\!\!&\!\!\textbf{85.05}$\pm$0.03\!\!&\!\!\textbf{89.24}$\pm$0.03\!\!\\ \cline{2-7}\Tstrut
&Places365&\!\!\textbf{50.08}$\pm$0.16\!\!&\!\!\textbf{59.27}$\pm$0.11\!\!&\!\!\textbf{77.22}$\pm$0.03\!\!&\!\!84.81$\pm$0.04\!\!&\!\!89.06$\pm$0.02\!\!\\ \bottomrule
\end{tabular}
\end{center}
\label{table:classification_performance_std}
\vspace*{-0.3cm}
\end{table}

\begin{table}[t!]
\caption{IoU and standard deviation\,($\%$) of \algnamea{} on CUB200\,(224$\times$224) and CAR\,(224$\times$224) under few-shot and full-shot learning settings.}
\small
\begin{center}
\begin{tabular}{X{1.1cm}|X{1.2cm}|X{1.39cm}X{1.39cm}X{1.39cm}|X{1.39cm}X{1.39cm}X{1.39cm}} \toprule
\multicolumn{2}{c|}{\multirow{2}{*}{Datasets}}&\multicolumn{3}{c|}{L1}&\multicolumn{3}{c}{L1-IoU}\\\cline{3-8}
\multicolumn{2}{c|}{} &\multicolumn{3}{c|}{\makecell[c]{\vspace*{-0.08cm}\# Examples ($N$)}}& \multicolumn{3}{c}{\makecell[c]{\vspace*{-0.08cm}\# Examples ($N$)}}\\ \midrule
In-dist.& \!\!\!OOD\!\!\!& \!\!\!2,000\!\!\! &  \!\!\!4,000\!\!\! & \!\!\!Full\!\!\! & \!\!\!2,000\!\!\!&\!\!\!4,000\!\!\! & Full \\ \midrule
\multirow{2}{*}{\vspace*{-0.cm}\makecell[c]{\!\!CUB200\!\!\\ \!\!\!\!(224$\times$224)\!\!\!\!}}
& \!\!\!{ImageNet}\!\!\! & \!\!\textbf{67.16}$\pm$0.05\!\! & \!\!\textbf{74.31}$\pm$0.03\!\! & \!\!\textbf{77.12}$\pm$0.02\!\! & \!\!\textbf{67.22}$\pm$0.02\!\! & \!\!\textbf{74.40}$\pm$0.04\!\! & \!\!\textbf{77.24}$\pm$0.03\!\! \\ \cline{2-8}\Tstrut
& \!\!\!{Places365}\!\!\!& \!\!66.70$\pm$0.07\!\! & \!\!73.55$\pm$0.05\!\! & \!\!76.86$\pm$0.03\!\! & \!\!66.87$\pm$0.10\!\! & \!\!73.63$\pm$0.05\!\! & \!\!77.01$\pm$0.04\!\! \\ \midrule
\multirow{2}{*}{\vspace*{-0.cm}\makecell[c]{\!\!CAR\!\!\\ \!\!\!\!(224$\times$224)\!\!\!\!}}
&\!\!\!{ImageNet}\!\!\!&\!\!\textbf{85.23}$\pm$0.04\!\! & \!\!\textbf{87.82}$\pm$0.02\!\! & \!\!\textbf{91.32}$\pm$0.01\!\!&\!\!\textbf{85.82}$\pm$0.05\!\!& \!\!\textbf{89.11}$\pm$0.04\!\! & \!\!\textbf{91.40}$\pm$0.03\!\!\\ \cline{2-8}\Tstrut
&\!\!\!{Places365}\!\!\!& \!\!84.26$\pm$0.06\!\! & \!\!87.59$\pm$0.07\!\! & \!\!90.86$\pm$0.02\!\! & \!\!84.73$\pm$0.05\!\! & \!\!88.83$\pm$0.04\!\! & \!\!91.28$\pm$0.02\!\!\\ \bottomrule
\end{tabular}
\end{center}
\label{table:bbox_iou_std}
\vspace*{-0.2cm}
\end{table}

\begin{table}[t!]
\caption{GT-known Loc and standard deviation of \algnamea{} on CUB200\,(224$\times$224) and CAR (224$\times$224) under few-shot and full-shot learning settings.}
\begin{center}
\small
\begin{tabular}{X{2cm} |X{2cm} |X{1.6cm} X{1.6cm} X{1.6cm}} \toprule
\multicolumn{2}{c|}{{Datasets}} & \multicolumn{3}{c}{{\# Examples ($N$)}} \\\cline{1-2}\cline{3-5}\Tstrut
In-dist. & Out-of-dist. & 2,000 &  4,000 & Full-shot \\ \midrule
% contetns
\multirow{2}{*}{\vspace*{-0.25cm}\makecell[c]{CUB200\\ (224$\times$224)}}
& ImageNet &\textbf{59.68}$\pm$0.07&\textbf{61.88}$\pm$0.04&\textbf{65.56}$\pm$0.05\\ \cline{2-5}\Tstrut 
& Places365 &58.24$\pm$0.09&60.90$\pm$0.05&64.84$\pm$0.04\\ \midrule
\multirow{2}{*}{\vspace*{-0.25cm}\makecell[c]{CAR\\ (32$\times$32)}}
&ImageNet&\textbf{65.82}$\pm$0.10&\textbf{69.05}$\pm$0.07&\textbf{72.14}$\pm$0.02\\\cline{2-5}\Tstrut
&Places365&65.70$\pm$0.08&67.64$\pm$0.06&71.62$\pm$0.02\\ \bottomrule
\end{tabular}
\end{center}
\label{table:GT_known_Loc_std}
\vspace*{-0.1cm}
\end{table}
