# Supplementary material for: Prioritizing Informative Features and Examples for Deep Learning from Noisy Data
Source: arXiv:2403.00013 source file (2024-08-12)
Supplement: Supplementary file 2 [file 7_appendix.tex]

\section{Supplementary Material}

\subsubsection{Standard Deviations of Main Results}
{
Table~\ref{table:overall_performance_withstd} repeats Table~\ref{table:overall_performance} with the addition of the standard deviations. Note that the standard deviations are very small, and the significance of the empirical results is sufficiently high.}

\newpage
\begin{landscape}
\begin{table}[t!]
\caption{Last test accuracy ($\%$) at the final round {with the standard deviations} for CIFAR10, CIFAR100, and ImageNet.}
\label{table:overall_performance_withstd}
\vspace{-0.05cm}
\begin{center}
\scriptsize
\begin{tabular}{c|c|c c c c|c c c c|c c c c} \toprule
\multicolumn{2}{c|}{Datasets}&\multicolumn{4}{c|}{CIFAR10 (4:6 split)}&\multicolumn{4}{c|}{CIFAR100 (40:60 split)}&\multicolumn{4}{c}{ImageNet (50:950 split)}\\\hline \addlinespace[0.15ex]
\multicolumn{2}{c|}{Noise Ratio} &\!10$\%$\!&\!20$\%$\!&\!40$\%$\!&\!60$\%$\!&\!10$\%$\!&\!20$\%$\!&\!40$\%$\!&\!60$\%$\!&\!10$\%$\!&\!20$\%$\!&\!40$\%$\!&\!60$\%$\!\\ \addlinespace[0.15ex]\hline\addlinespace[0.3ex]
{Non-AL}&{RANDOM}&\!{89.83{\tiny $\pm$0.61}}\!&\!{89.06{\tiny $\pm$0.59}}\!&\!{87.73{\tiny $\pm$0.83}}\!&\!{85.64{\tiny $\pm$0.90}}\!&\!{60.88{\tiny $\pm$0.67}}\!&\!{59.69{\tiny $\pm$0.61}}\!&\!{55.52{\tiny $\pm$0.46}}\!&\!{47.37{\tiny $\pm$0.80}}\!&\!{62.72{\tiny $\pm$0.68}}\!&\!{60.12{\tiny $\pm$0.23}}\!&\!{54.04{\tiny $\pm$0.56}}\!&\!{48.24{\tiny $\pm$0.62}}\!\\\cline{1-14}\Tstrut
\multirow{4}{*}{\vspace{-0.15cm}\makecell[c]{Standard\\AL}}&CONF&\!92.83{\tiny $\pm$0.49}\!&\!91.72{\tiny $\pm$0.55}\!&\!88.69{\tiny $\pm$0.75}\!&\!85.43{\tiny $\pm$0.82}\!&\!62.84{\tiny $\pm$0.52}\!&\!60.20{\tiny $\pm$0.79}\!&\!53.74{\tiny $\pm$0.38}\!&\!45.38{\tiny $\pm$0.64}\!&\!63.56{\tiny $\pm$0.34}\!&\!62.56{\tiny $\pm$0.56}\!&\!51.08{\tiny $\pm$0.63}\!&\!45.04{\tiny $\pm$0.90}\!\\\cline{2-14}\Tstrut
&CORESET&\!91.76{\tiny $\pm$0.55}\!&\!91.06{\tiny $\pm$0.57}\!&\!89.12{\tiny $\pm$0.72}\!&\!86.50{\tiny $\pm$0.79}\!&\!63.79{\tiny $\pm$0.45}\!&\!62.02{\tiny $\pm$0.54}\!&\!56.21{\tiny $\pm$0.43}\!&\!48.33{\tiny $\pm$0.51}\!&\!63.64{\tiny $\pm$0.60}\!&\!\underline{62.24}{\tiny $\pm$0.23}\!&\!55.32{\tiny $\pm$0.56}\!&\!49.04{\tiny $\pm$0.42}\!\\\cline{2-14}\Tstrut
&LL&\!92.09{\tiny $\pm$0.57}\!&\!91.21{\tiny $\pm$0.57}\!&\!\underline{89.41}{\tiny $\pm$0.62}\!&\!86.95{\tiny $\pm$0.58}\!&\!\underline{65.08}{\tiny $\pm$0.54}\!&\!\underline{64.04}{\tiny $\pm$0.48}\!&\!56.27{\tiny $\pm$0.53}\!&\!48.49{\tiny $\pm$0.57}\!&\!63.28{\tiny $\pm$0.23}\!&\!61.56{\tiny $\pm$0.46}\!&\!55.68{\tiny $\pm$0.60}\!&\!47.30{\tiny $\pm$0.72}\!\\\cline{2-14}\Tstrut
&BADGE&\!\underline{92.80}{\tiny $\pm$0.49}\!&\!\underline{91.73}{\tiny $\pm$0.45}\!&\!89.27{\tiny $\pm$0.54}\!&\!86.83{\tiny $\pm$0.38}\!&\!62.54{\tiny $\pm$0.47}\!&\!61.28{\tiny $\pm$0.43}\!&\!55.07{\tiny $\pm$0.52}\!&\!47.60{\tiny $\pm$0.42}\!&\!\underline{64.84}{\tiny $\pm$0.25}\!&\!61.48{\tiny $\pm$0.29}\!&\!54.04{\tiny $\pm$0.56}\!&\!47.80{\tiny $\pm$0.47}\!\\\cline{1-14}\Tstrut
\multirow{2}{*}{\makecell[c]{Open-set\\AL}}&CCAL&\!90.55{\tiny $\pm$0.35}\!&\!89.99{\tiny $\pm$0.45}\!&\!88.87{\tiny $\pm$0.70}\!&\!\underline{87.49}{\tiny $\pm$0.75}\!&\!61.20{\tiny $\pm$0.39}\!&\!61.16{\tiny $\pm$0.57}\!&\!\underline{56.70}{\tiny $\pm$0.56}\!&\!50.20{\tiny $\pm$0.49}\!&\!61.68{\tiny $\pm$0.26}\!&\!60.70{\tiny $\pm$0.38}\!&\!\underline{56.60}{\tiny $\pm$0.85}\!&\!51.16{\tiny $\pm$0.74}\!\\\cline{2-14}\Tstrut
&SIMILAR&\!89.92{\tiny $\pm$0.55}\!&\!89.19{\tiny $\pm$0.59}\!&\!88.53{\tiny $\pm$0.66}\!&\!87.38{\tiny $\pm$0.73}\!&\!60.07{\tiny $\pm$0.35}\!&\!59.89{\tiny $\pm$0.53}\!&\!56.13{\tiny $\pm$0.41}\!&\!\underline{50.61}{\tiny $\pm$0.34}\!&\!63.92{\tiny $\pm$0.20}\!&\!61.40{\tiny $\pm$0.36}\!&\!56.48{\tiny $\pm$0.78}\!&\!\underline{52.84}{\tiny $\pm$0.62}\!\\\cline{1-14} \Tstrut
Proposed&\textbf{MQ-Net}&\!\textbf{93.10}{\tiny $\pm$0.40}\!&\!\textbf{92.10}{\tiny $\pm$0.45}\!&\!\textbf{91.48}{\tiny $\pm$0.56}\!&\!\textbf{89.51}{\tiny $\pm$0.58}\!&\!\textbf{66.44}{\tiny $\pm$0.55}\!&\!\textbf{64.79}{\tiny $\pm$0.44}\!&\!\textbf{58.96}{\tiny $\pm$0.36}\!&\!\textbf{52.82}{\tiny $\pm$0.46}\!&\!\textbf{65.36}{\tiny $\pm$0.42}\!&\!\textbf{63.08}{\tiny $\pm$0.23}\!&\!\textbf{56.95}{\tiny $\pm$0.56}\!&\!\textbf{54.11}{\tiny $\pm$0.45}\!\\\hline\addlinespace[0.3ex]
\multicolumn{2}{c|}{\emph{$\%$ improve over 2nd best}}&0.32&0.40&2.32&2.32&2.09&1.17&3.99&4.37&0.80&1.35&0.62&2.40\\\hline
\multicolumn{2}{c|}{\emph{$\%$ improve over the least}}&3.53&3.26&3.33&4.78&10.6&8.18&9.71&16.39&5.97&3.92&11.49&20.14\\\bottomrule
\end{tabular}
\end{center}
\vspace*{-0.4cm}
\end{table}

\end{landscape}
