# Supplementary material for: Prioritizing Informative Features and Examples for Deep Learning from Noisy Data
Source: arXiv:2403.00013 source file (2024-08-12)
Supplement: Supplementary file 3 [file 7-appendix.tex]

\begin{appendices}
\section{Proof of Theorem 3.3}
\label{appendix:proof_theory3.3}
3.1 Reduced Neighborhood Confidence part
about line 165

\section{Details for $\text{\algname{}}_B$}
\label{appendix:detail_OursB}
3.2 Data Pruning by Maximizing Neighborhood Confidence Coverage
about line 215

\section{Proof of Theorem 3.4}
\label{appendix:proof_theory3.4}
3.2 Data Pruning by Maximizing Neighborhood Confidence Coverage 
Optimization with Greedy Approximation.
about line 227

\section{Implementation Detail}
\label{appendix:implementation_detail}
4.1 Experiment Setting 
Implementation Details
about line 277

\section{Limitation and Potential Negative Societal Impact}
\label{appendix:limitation}
\noindent\textbf{Limitation.}
While \algname{} has demonstrated consistent effectiveness in handling classification tasks using various real-world noisy datasets, it is crucial to validate its applicability across a broader spectrum of tasks, including object localization and natural language processing.
This verification would be valuable because the need for data pruning in the face of label noise is consistently high across a wide range of real-world tasks. 
On the other hand, the principle of \algname{} has the potential to advance other realistic learning scenarios, such as continual learning and active learning. In these scenarios, an efficient selection of informative examples is equally important, and we consider it valuable for future research.

\smallskip
\noindent\textbf{Potential Negative Societal Impact.} 
% robust deep learning -> generally neglect efficiency and thus criticized for being environmentally unfriendly
% In this regard, ours, as data pruning, -> leads to the full potential of state-of-the-art Re-labeling with relieving the enormous computational cost
% As a result, our work would contribute to an environmentally friendness rather than negative societal impact 
In general, the learning pipeline of robust deep learning has primarily focused on enhancing its resilience to label noise, often neglecting the efficiency of the algorithm itself. This approach has drawn criticism for its substantial energy consumption and resulting negative environmental impact. In this regard, \algname{}, as a data pruning technique, alleviates the significant computational costs associated with robust deep learning while still harnessing the full potential of state-of-the-art re-labeling methods. By reducing computational requirements, we believe that our work can contribute to an environmentally friendly approach, mitigating the potential negative societal impact associated with energy-intensive algorithms.

\end{appendices}
